# Supplementary material for: Approximating Persistent Homology in Euclidean Space Through Collapses
Source: arXiv:1403.0533 source file (2014-08-20)
Supplement: Supplementary file 1 [file appendix.tex]

\appendix
\section{The Sandwich Theorem}
\teo{The families of homomorphisms $\{\phi_\alpha\}_{\alpha\in\mathbb{R}}$ and $\{\psi_\alpha\}_{\alpha\in\mathbb{R}}$ satisfy the diagrams of Definition 3. In particular, the persistence modules $\left(H_p(\mathcal{C}_\mathcal{U}), \eta_{\mathcal{U}(-)}^{\mathcal{U}(-)}\right)$ and $\left(H_p(\mathcal{C}_\mathcal{V}), \eta_{\mathcal{V}(-)}^{\mathcal{V}(-)}\right)$ are $c$-approximate.}
\begin{proof}
\begin{align*}
\phi_{\alpha^\prime}\circ\eta_{\mathcal{U}(\alpha)}^{\mathcal{U}(\alpha^\prime)}\circ \psi_{\alpha/c} &= \eta_{\mathcal{U}(\alpha^\prime)}^{\mathcal{V}(c\alpha^\prime)}\circ \eta_{\mathcal{U}(\alpha)}^{\mathcal{U}(\alpha^\prime)}\circ (\pi_2 \circ \pi_1^{-1})_* \circ \left({\rm inc}_{W(\alpha/c)}^{U(\alpha)}\right)_*\circ (\pi_2 \circ \pi_1^{-1})^{-1}_*\circ \eta_{\mathcal{V}(\alpha/c)}^{\mathcal{W}(\alpha/c)}\\
&\stackrel{\text{\ref{eq:associative}}}{=} \eta_{\mathcal{U}(\alpha)}^{\mathcal{V}(c\alpha^\prime)}\circ (\pi_2 \circ \pi_1^{-1})_* \circ \left({\rm inc}_{W(\alpha/c)}^{U(\alpha)}\right)_*\circ (\pi_2 \circ \pi_1^{-1})^{-1}_*\circ \eta_{\mathcal{V}(\alpha/c)}^{\mathcal{W}(\alpha/c)}\\
&\stackrel{\text{\ref{eq:commutative}}}{=} (\pi_2 \circ \pi_1^{-1})_*\circ \left({\rm inc}_{U(\alpha)}^{V(c\alpha^\prime)}\right)_*\circ \left({\rm inc}_{W(\alpha/c)}^{U(\alpha)}\right)_*\circ (\pi_2 \circ \pi_1^{-1})^{-1}_*\circ \eta_{\mathcal{V}(\alpha/c)}^{{\mathcal{W}}(\alpha/c)}\\
&\stackrel{\text{\ref{eq:commutative}}}{=} \eta_{\mathcal{W}(\alpha/c)}^{\mathcal{V}(c\alpha^\prime)}\circ \eta_{\mathcal{V}(\alpha/c)}^{{{\mathcal{W}}(\alpha/c)}} \stackrel{\text{\ref{eq:commutative}}}{=} \eta_{\mathcal{V}(\alpha/c)}^{\mathcal{V}(c\alpha^\prime)}
\end{align*}

\begin{align*}
\phi_{\alpha^\prime}\circ\eta_{{\mathcal{U}}(\alpha)}^{{\mathcal{U}}(\alpha^\prime)} &= \eta_{\mathcal{U}(\alpha^\prime)}^{\mathcal{V}(c\alpha^\prime)}\circ \eta_{{\mathcal{U}}(\alpha)}^{{\mathcal{U}}(\alpha^\prime)} = \eta_{\mathcal{U}(\alpha)}^{\mathcal{V}(c\alpha^\prime)}\\
 &= (\pi_2\circ\pi_{-1})_*\circ\left({\rm inc}_{U(\alpha)}^{V(c\alpha^\prime)}\right)_*\circ (\pi_2\circ\pi_1^{-1})_*^{-1}\\
 &= (\pi_2\circ\pi_{-1})_*\circ \left({\rm inc}_{V(c\alpha)}^{V(c\alpha^\prime)}\right)_*\circ\left({\rm inc}_{U(\alpha)}^{V(c\alpha)}\right)_*\circ (\pi_2\circ\pi_1^{-1})_*^{-1}\\
 &= \eta_{\mathcal{V}(c\alpha)}^{\mathcal{V}(c\alpha^\prime)}\circ (\pi_2\circ\pi_1^{-1})_* \circ \left({\rm inc}_{U(\alpha)}^{V(c\alpha)}\right)_*\circ (\pi_2\circ\pi_1^{-1})_*^{-1}\\
 &= \eta_{\mathcal{V}(c\alpha)}^{\mathcal{V}(c\alpha^\prime)}\circ \eta_{\mathcal{U}(\alpha)}^{\mathcal{V}(c\alpha)} = \eta_{\mathcal{V}(c\alpha)}^{\mathcal{V}(c\alpha^\prime)}\circ \phi_{\alpha}
\end{align*}
\end{proof}
